# Supplementary material for: Decay Rate of Magnetic Dipoles near Non-magnetic Nanostructures
Source: arXiv:1707.07006 ancillary file (2018-01-23)
Supplement: Supplementary file 1 [file 2017-decay-magnetic-dipole_supporting_info.pdf]

# Supporting Informations: Decay Rate of Magnetic Dipoles near Non–magnetic Nanostructures

Peter R. Wiecha,[1,*] Arnaud Arbouet,[1] Aurélien Cuche,[1] Vincent Paillard,[1] and Christian Girard[1]
[1] *CEMES-CNRS, Université de Toulouse, CNRS, UPS, Toulouse, France*

## I. DETAILS ON COUPLED MODEL

### A. Field susceptibility for the magnetic field

An oscillating (at frequency $\omega_0$) magnetic dipole at $\mathbf{r}_0$ creates an electro-magnetic field at $\mathbf{r}$ whose electric component writes

$$\mathbf{E}_0(\mathbf{r},\omega_0) = ik_0 \nabla_{\mathbf{r}} \wedge \mathcal{G}_0(\mathbf{r},\mathbf{r}_0,\omega_0) \cdot \mathbf{m}(\omega_0) \tag{S.1}$$

Above, $\omega_0 = ck_0$ and $\mathcal{G}_0$ is the Green's function in vacuum

$$\mathcal{G}_0(\mathbf{r},\mathbf{r}_0,\omega_0) = \frac{\exp(ik_0|\mathbf{r}-\mathbf{r}_0|)}{|\mathbf{r}-\mathbf{r}_0|}. \tag{S.2}$$

From this, we can define a field susceptibility for the electric component of the magnetic dipole's emission (see also Ref. S1, Eqs. 4.5 and 4.6):

$$S^{EH}(\mathbf{r},\mathbf{r}_0,\omega_0) = ik_0 \nabla \wedge \mathcal{G}_0(\mathbf{r},\mathbf{r}_0,\omega_0)\,, \tag{S.3}$$

hence

$$\mathbf{E}_0(\mathbf{r},\omega_0) = \mathcal{S}^{EH}(\mathbf{r},\mathbf{r}_0,\omega_0) \cdot \mathbf{m}(\omega_0)\ . \tag{S.4}$$

Omitting the dependence on $\mathbf{r}, \mathbf{r}_0$ and $\omega_0$ of $\mathcal{G}_0$, this explicitly writes (see also Ref. S2)

$$\mathcal{S}^{EH}(\mathbf{r},\mathbf{r}_0,\omega_0) = ik_0 \begin{pmatrix} 0 & -\frac{\partial}{\partial z}\mathcal{G}_0 & +\frac{\partial}{\partial y}\mathcal{G}_0 \\ +\frac{\partial}{\partial z}\mathcal{G}_0 & 0 & -\frac{\partial}{\partial x}\mathcal{G}_0 \\ -\frac{\partial}{\partial y}\mathcal{G}_0 & +\frac{\partial}{\partial x}\mathcal{G}_0 & 0 \end{pmatrix}\ . \tag{S.5}$$

The electric field (Eq. (S.4)) can couple to a nano-structure (permittivity $\epsilon_r \neq 1$, permeability $\mu_r = 1$). Using the concept of a generalized propagator, the full local electric field can be written[S3]

$$\mathbf{E}(\mathbf{r},\omega_0) = \int_V \mathcal{K}(\mathbf{r},\mathbf{r}',\omega_0) \cdot \mathbf{E}_0(\mathbf{r}',\omega_0) \mathrm{d}\mathbf{r}', \tag{S.6}$$

where the integral runs over the volume $V$ of the nano-structure and $\mathcal{K}$ is the generalized field propagator. We can now calculate the response of the nano-structure to the *electric* field emitted by the *magnetic* dipole, *i.e.* the induced electric field at positions $\mathbf{r}_s$ inside the structure

$$\mathbf{E}(\mathbf{r}_s,\omega_0) = \int_V \mathcal{K}(\mathbf{r}_s,\mathbf{r}',\omega_0) \cdot \mathcal{S}^{EH}(\mathbf{r}',\mathbf{r}_0,\omega_0) \cdot \mathbf{m}(\omega_0) \mathrm{d}\mathbf{r}'\,. \tag{S.7}$$

The electric polarization $\mathbf{P}$ of the particle can be expressed by the field Eq. (S.7) as

$$\mathbf{P}(\mathbf{r}_s,\omega_0) = \chi(\mathbf{r}_s,\omega_0) \cdot \mathbf{E}(\mathbf{r}_s,\omega_0)\,, \tag{S.8}$$

* e-mail : peter.wiecha@cemes.fr

and using an appropriate propagator $\mathcal{S}^{HE}$ (see Ref. S2), the electric field at a position $\mathbf{r}$ outside the structure, induced by the particle's electric polarization, can be obtained by the following equation:

$$\mathbf{H}(\mathbf{r},\omega_0) = \int_V \mathcal{S}^{HE}(\mathbf{r},\mathbf{r}',\omega_0)\cdot\mathbf{P}(\mathbf{r}',\omega_0)\mathrm{d}\mathbf{r}' \,, \tag{S.9}$$

where $\mathcal{S}^{HE} = -\mathcal{S}^{EH}$.

Inserting equation (S.7) in equation (S.9), we now have an expression for the magnetic field, induced by a magnetic dipole in the presence of an arbitrary nanostructure:

$$\mathbf{H}(\mathbf{r},\omega_0) = \int_V \mathrm{d}\mathbf{r}' \int_V \mathcal{S}^{HE}(\mathbf{r},\mathbf{r}',\omega_0)\cdot\chi(\mathbf{r}',\omega_0)\cdot\mathcal{K}(\mathbf{r}',\mathbf{r}'',\omega_0)\cdot\mathcal{S}^{EH}(\mathbf{r}'',\mathbf{r}_0,\omega_0)\cdot\mathbf{m}\,\mathrm{d}\mathbf{r}'' \tag{S.10}$$

from which we define the field-susceptibility of the magnetic field

$$S_p^{HH}(\mathbf{r},\mathbf{r}',\omega_0) = \int_V \mathrm{d}\mathbf{r}' \int_V \mathcal{S}^{HE}(\mathbf{r},\mathbf{r}',\omega_0)\cdot\chi(\mathbf{r}',\omega_0)\cdot\mathcal{K}(\mathbf{r}',\mathbf{r}'',\omega_0)\cdot\mathcal{S}^{EH}(\mathbf{r}'',\mathbf{r}_0,\omega_0)\,\mathrm{d}\mathbf{r}'' \,. \tag{S.11}$$

The subscript $p$ indicates that the field-susceptibility accounts for an effect due to a polarizable nanostructure. By discretizing the double integral in Eq. (S.11) (via cubic meshing of the nano-particle), the $(3\times3)$ tensor $S_p^{HH}$ can be calculated for any position $\mathbf{r}_0$ of a magnetic dipole transition in the vicinity of a nano-particle of arbitrary shape.

### B. Magnetic dipole decay-rate $\Gamma_m$

The decay rate of an electric dipole transition (dipole moment $\boldsymbol{\mu}$), coupled to a nanostructure writes[S4]

$$\Gamma_\mu(\mathbf{r}_0,\omega_0) = \frac{2|\boldsymbol{\mu}|^2}{\hbar}\mathbf{u}\cdot\mathrm{Im}\big(S^{EE}(\mathbf{r}_0,\mathbf{r}_0,\omega_0)\big)\cdot\mathbf{u}\,, \tag{S.12}$$

where $\hbar$ is the reduced Planck quantum, $\mathbf{u}$ the unitary vector in direction of $\boldsymbol{\mu}$ and $S^{EE}$ the electric field susceptibility

$$S^{EE} = S_0^{EE} + S_p^{EE}\,, \tag{S.13}$$

composed of a vacuum contribution (subscript 0) and one due to the presence of the nano-structure (subscript $p$). Likewise, we can write the decay-rate of the magnetic dipole

$$\Gamma_m(\mathbf{r}_0,\omega_0) = \frac{2|\mathbf{m}|^2}{\hbar}\mathbf{u}\cdot\mathrm{Im}\big(S^{HH}(\mathbf{r}_0,\mathbf{r}_0,\omega_0)\big)\cdot\mathbf{u} \tag{S.14}$$

$$= \Gamma_m^0 + \frac{3}{2k_0^3}\Gamma_m^0\;\mathbf{u}\cdot\mathrm{Im}\big(S_p^{HH}(\mathbf{r}_0,\mathbf{r}_0,\omega_0)\big)\cdot\mathbf{u} \tag{S.15}$$

where

$$S^{HH} = S_0^{HH} + S_p^{HH} \tag{S.16}$$

and the vacuum rate given by $S_0^{HH}$ gives, in analogy to an electric dipole transition[S4]

$$\Gamma_m^0 = \frac{4|\mathbf{m}|^2k_0^3}{3\hbar}\,. \tag{S.17}$$

Inserting $S_p^{HH}$ from Eq. (S.11) together with Eq. (S.17) into Eq. (S.15) finally yields the dipole's decay rate relative to the vacuum value.

*Note:* The decay rate of an electric dipole emitter can be numerically implemented in the exact same way, by replacing the electric field emitted by the magnetic dipole (Eq. (S.1)) by the electric field emitted by an electric dipole, at the beginning of the derivation. It writes:

$$\mathbf{E}_0(\mathbf{r},\omega_0) = \{\mathbf{I}k_0^2 + \nabla_\mathbf{r}\nabla_\mathbf{r}\}\mathcal{G}_0(\mathbf{r},\mathbf{r}_0,\omega_0)\cdot\boldsymbol{\mu}(\omega_0)\,, \tag{S.18}$$

## II. COMPARISON ANALYTICAL MODEL, COUPLED MODEL

We compare the analytical model describing the decay of magnetic dipoles with the coupled implementation for nanoparticles of arbitrary shape. The analytical model is valid only for sufficiently large distances to very small spherical dielectric particles with close to no physical extension. The coupled model on the other hand allows to describe complex nano-structures of arbitrary geometry via a volume discretization scheme and can be used with good accuracy close to the surface of large particles.

### A. Single dielectric sphere

To compare the analytical and coupled approaches, we calculate the decay of a magnetic dipole emitter at a plane 20 nm above a small dielectric sphere. The sphere is modeled in the analytical method by a polarizability of $\alpha_e = r^3\,(\epsilon - 1)/(\epsilon + 2) \approx 1688\,\text{nm}^3$, obtained for a radius $r = 15\,\text{nm}$ and an optical index $n = 2$. In the coupled method, we describe the sphere using $3 \times 3 \times 3$ meshpoints of 10 nm stepsize, resulting in a block of 30 nm edge length (approximating a sphere of radius $r = 15\,\text{nm}$). The refractive index is $n = 2.0$, which results in a total polarizability of approximately equal value compared to the analytical model. In both cases the dipole emits at a wavelength $\lambda_0 = 500\,\text{nm}$.

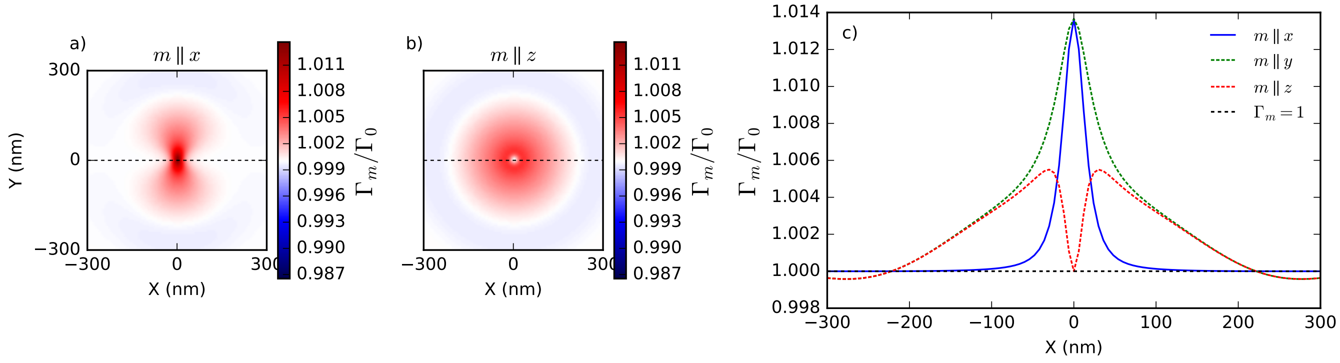


FIG. S.1. Analytic model: single dielectric sphere at 0, 0, 0. Polarizability $\alpha_e = 1688\,\text{nm}^3$ (corresponding to $r = 15\,\text{nm}$, $n = 2.0$). a) dipole $\parallel x$, b) dipole $\parallel z$ and c) profiles along $x$ ($y = 0$) at $z_0 = 20\,\text{nm}$ above the sphere center.

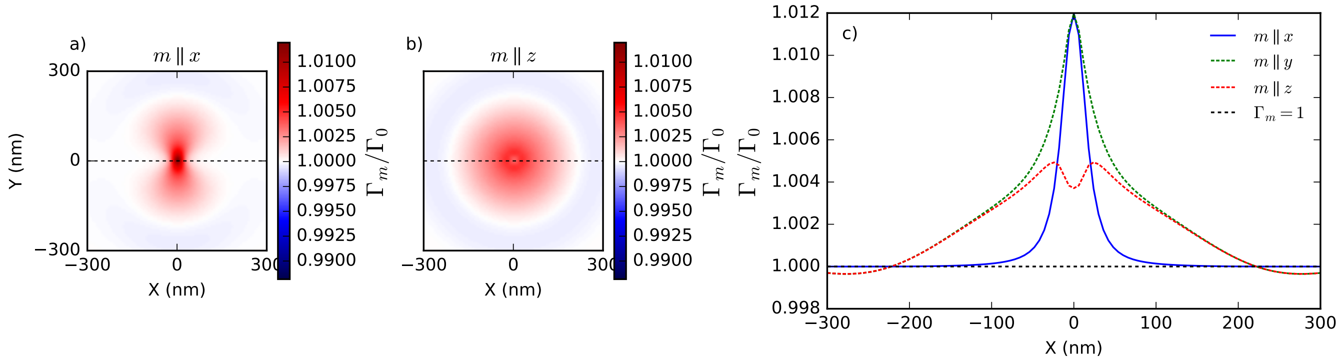


FIG. S.2. Coupled model: single dielectric "sphere" at 0, 0, 0. Radius $r = 15\,\text{nm}$, $n = 2.0$ composed of $3 \times 3 \times 3$ meshpoints. a) dipole $\parallel x$, b) dipole $\parallel z$ and c) profiles along $x$ ($y = 0$) at $z_0 = 20\,\text{nm}$ above the sphere center.

As shown in figure S.1 (analytical) and figure S.2 (coupled), both approaches yield an excellent agreement. The only visible difference is a slightly smaller decay rate in the coupled model, which we attribute to the finite physical extension of the material compared to the infinitely small sphere in the analytical case. The fact that on top of the sphere the decay rate $\Gamma_m/\Gamma_0 \neq 1$ of a dipole $m$ along $z$, is also a result of the non-zero dimension of the particle in the coupled approach.

### B. Several dielectric spheres

In figures S.3 and S.4 we show the same kind of simulation as above, but instead of a single dielectric sphere, we calculate the case of ten spheres randomly distributed on the $XY$ plane. Again, we obtain an excellent agreement between analytical and coupled model.

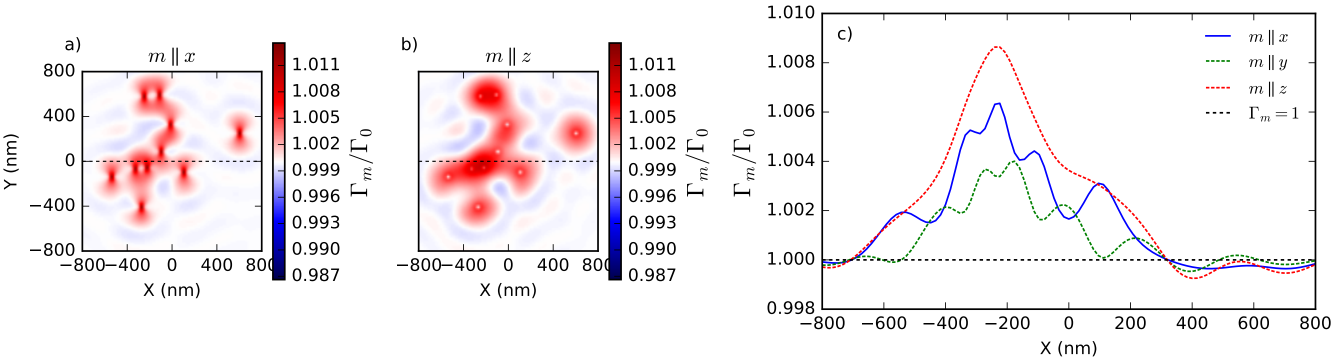


FIG. S.3. Analytic model: several dielectric spheres on the $XY$ plane, each of polarizability $\alpha_e = 1688\,\text{nm}^3$ (corresponding to $r = 15\,\text{nm}$, $n = 2.0$). a) dipole $\parallel x$, b) dipole $\parallel z$ and c) profiles along $x$ ($y = 0$) at $z_0 = 20\,\text{nm}$ above the sphere center.

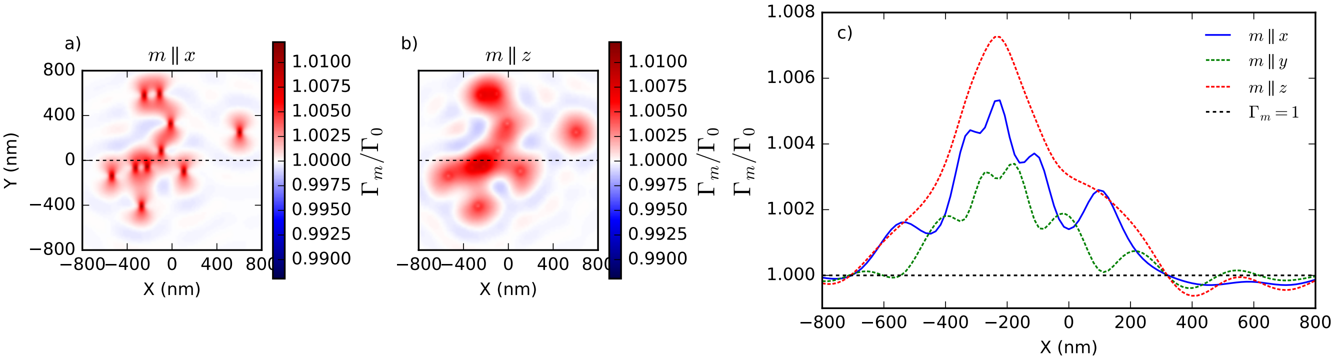


FIG. S.4. Coupled model: 10 dielectric "spheres" randomly distributed on the $XY$ plane, each of radius $r = 15\,\text{nm}$, $n = 2.0$, composed of $3 \times 3 \times 3$ meshpoints. a) dipole $\parallel x$, b) dipole $\parallel z$ and c) profiles along $x$ ($y = 0$) at $z_0 = 20\,\text{nm}$ above the sphere center.

## III. COUPLED MODEL: MESHSIZE IMPACT

In order to assess the influence of the mesh stepsize on the decay rate calculations using the coupled model, we calculate the same decay rate mapping using different discretization stepsizes. As structure we use again the corral structure composed of 20 $100 \times 100 \times 100\,\mathrm{nm}^3$ dielectric blocks ($n = 2$), separated by a distance of 100 nm, which we have already shown in figure 4 of the main paper. The corral is placed in vacuum and raster-scanned 30 nm above the top surface by a dipolar emitter, emitting at $\lambda_0 = 500\,\mathrm{nm}$. The two columns at the left hand side of figure S.5 show the case of an electric dipole (ED), either oriented along $X$ (very left) or along $Z$ (second left). The two right hand columns show a magnetic dipole (MD), either oriented along $X$ (second right) or along $Z$ (right).

Figure S.5a) shows results for a simulation using $6 \times 6 \times 6$ meshpoints for each block of the corral (stepsize 16.66 nm). In b), the blocks are discretized with $7 \times 7 \times 7$ meshpoints (stepsize 14.29 nm) and in c) using $8 \times 8 \times 8$ meshpoints (stepsize 12.50 nm).

All three cases yield almost exactly the same results, demonstrating the robustness of the coupled method.

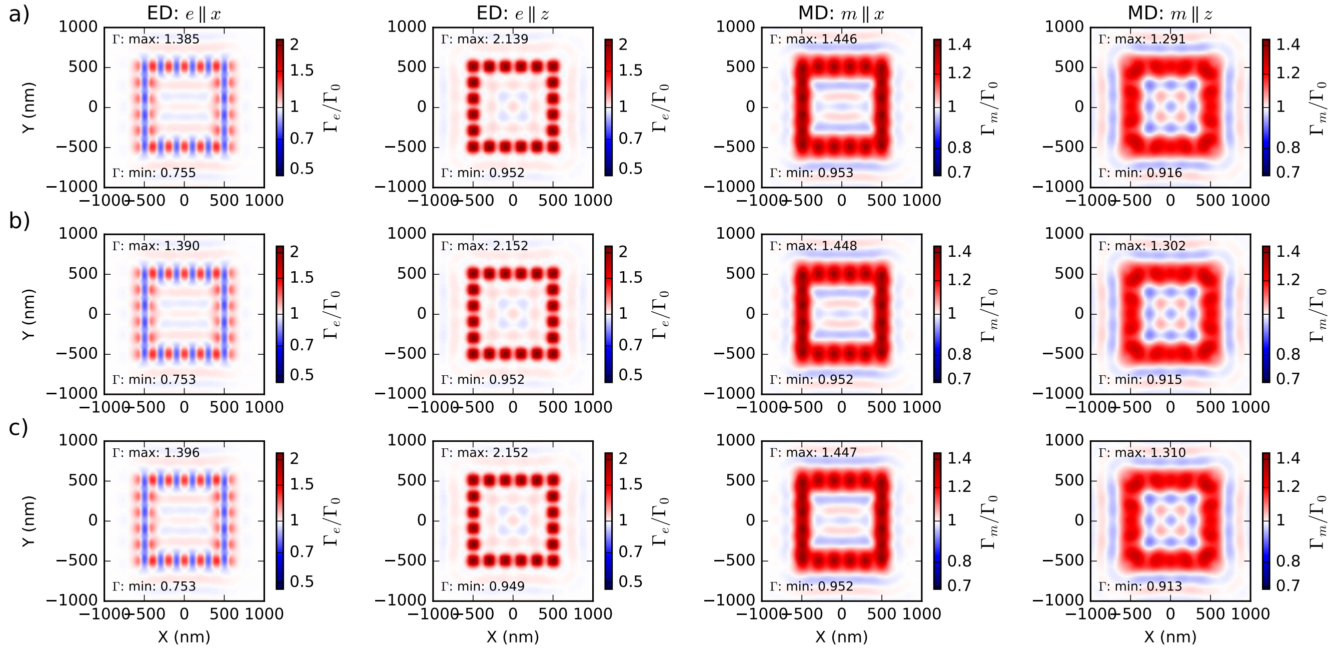


FIG. S.5. Maps of the decay rates of electric (ED, left: along $0X$, second left: along $0Z$) and magnetic dipoles (MD, second right: along $0X$, right: along $0Z$) 30 nm above a square corral of 20 dielectric nanocubes. The spacing between each cube of dimensions $100 \times 100 \times 100\,\mathrm{nm}^3$ is 100 nm, and the optical index is $n = 2.0$. Different discretization stepsizes where used: a) 16.66 nm, b) 14.29 nm and c) 12.50 nm.

## IV. COUPLED MODEL: IMPACT OF MATERIAL

To assess the impact of the refractive index on the decay rate and the confinement of the $\Gamma$-enhancement, we calculate the electric and magnetic decay rate above a dielectric corral structure for different refractive index. Figure S.6 shows the decay rate variations 30 nm above the corral for optical indices of the structure of a) $n = 1.5$, b) $n = 2.0$ and c) $n = 3.5$.

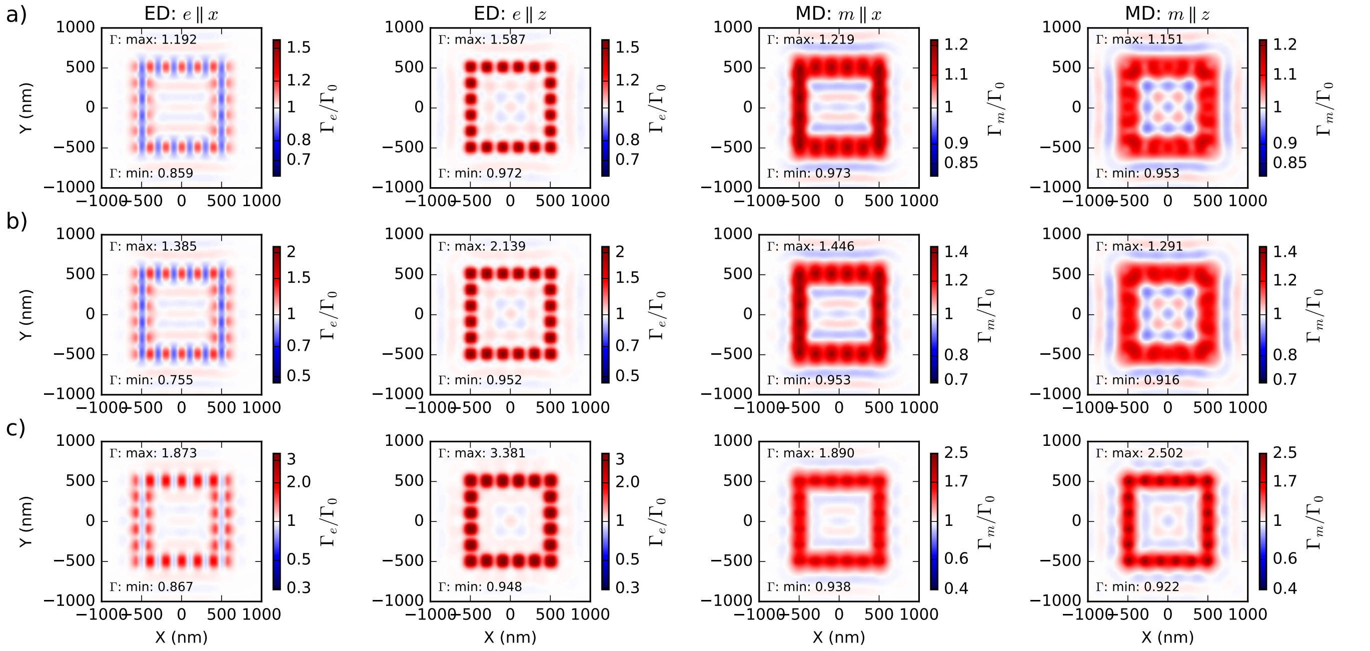


FIG. S.6. Maps of the decay rates of electric (ED, left: along $0X$, second left: along $0Z$) and magnetic dipoles (MD, second right: along $0X$, right: along $0Z$) 30 nm above a square corral of 20 dielectric nanocubes. The spacing between each cube of dimensions $100 \times 100 \times 100\,\mathrm{nm}^3$ is 100 nm using a discretization stepsize of 16.66 nm. The optical index is a) $n = 1.5$, b) $n = 2.0$ and c) $n = 3.5$.

## V. COUPLED MODEL: IMPACT OF RESONANCES

The corral structure acts like an optical resonator, so apart from the material of its building blocks, a possible resonant behavior can have an additional impact on the decay rates. In figures S.8-S.10 we show the decay rate along a line-scan through the center of the corral (at $Y = 0$), 30 nm above the upper surface, as a function of $X$-position and the dipole's emitting wavelength (see figure S.7). We calculated this data for optical indices of the structure of $n = 1.5$, $n = 2.0$ and $n = 3.5$ (figures S.8, S.9 and S.10, respectively).

We can summarize that although the effect of optical resonances is visible (mainly inside the corral), the influence of the material itself is dominating the change in decay rate.

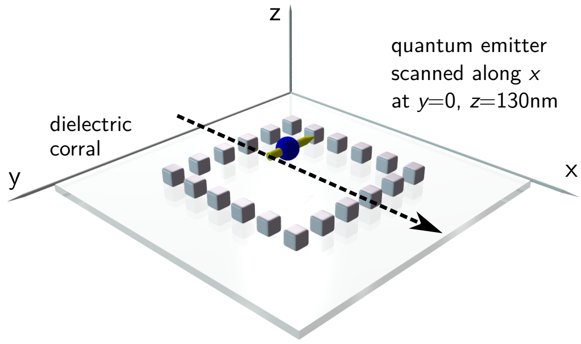


FIG. S.7. Sketch of the simulation: A dipolar emitter is scanned along $x$ ($y = 0$, $z = 130$ nm) above a corral composed of blocks of $100 \times 100 \times 100\,\text{nm}^3$ for different refractive indices. The simulation is repeated for different wavelengths to assess the spectral variations of the decay rate.

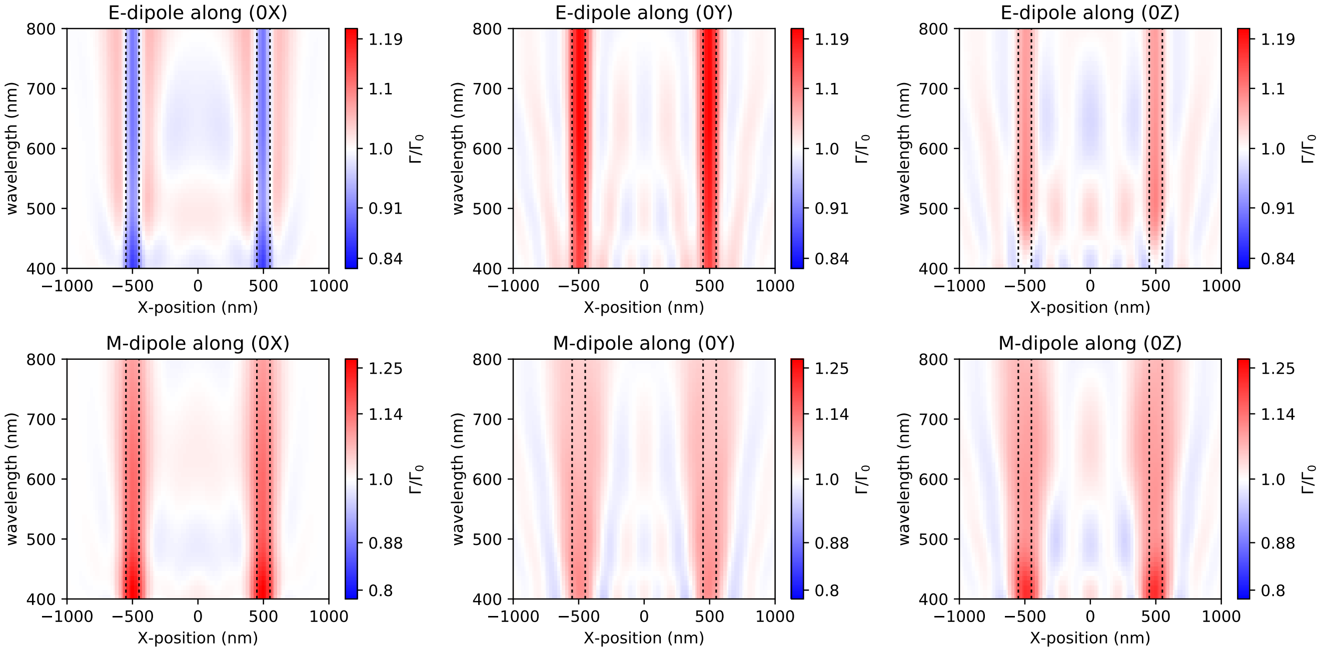


FIG. S.8. Decay rate of an electric (top row) and a magnetic (bottom row) dipole, scanned along $X$ through the center of a corral structure as a function of $X$-position and wavelength (same structure as used in figs. S.5 and S.6). The refractive index of the $100 \times 100 \times 100\,\text{nm}^3$ blocks is $n = 1.5$. The dipole orientation is (from left to right) along $0X$, $0Y$ and $0Z$. The borders of the corral blocks are indicated by dashed black lines.

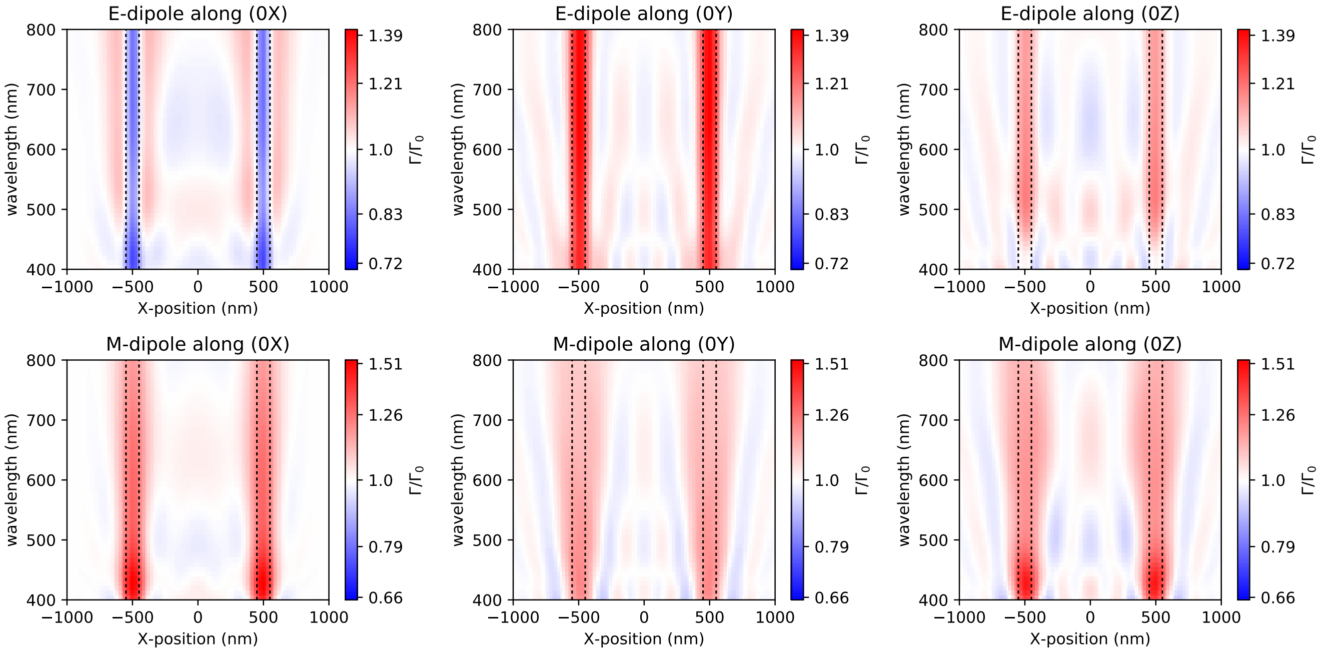


FIG. S.9. Same as fig. S.8 except with an optical index of $n = 2.0$.

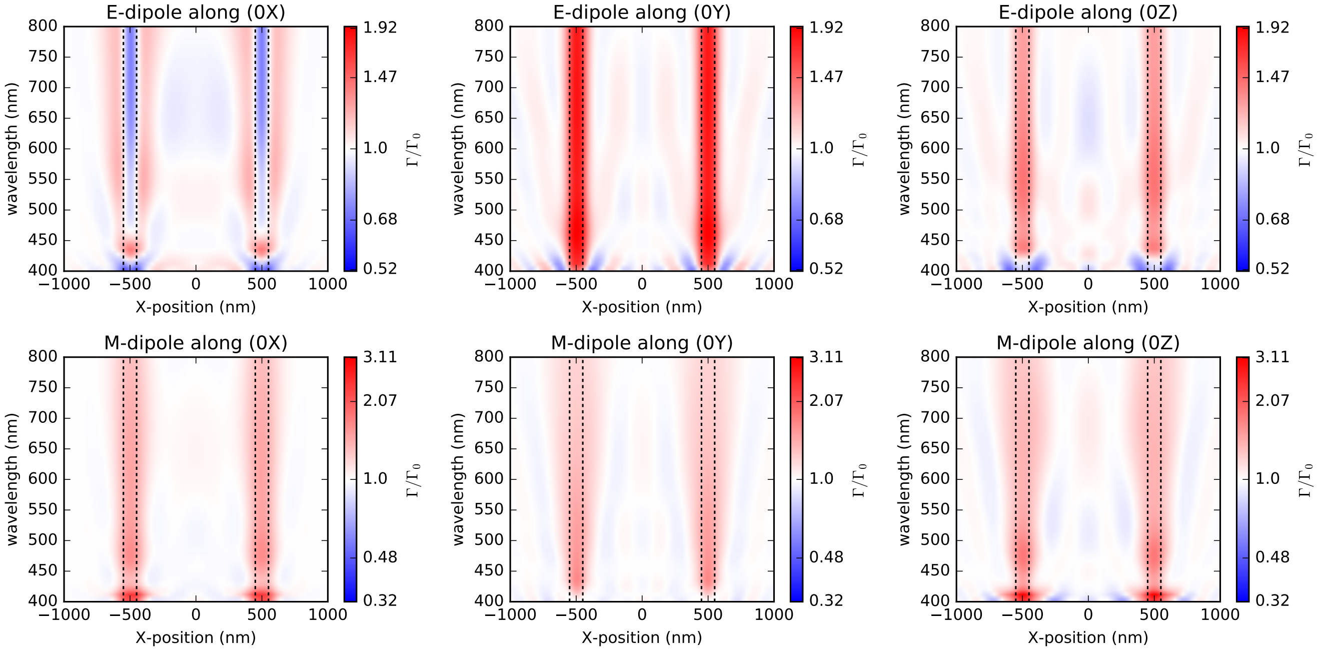


FIG. S.10. Same as fig. S.8 except with an optical index of $n = 3.5$.

## VI. TECHNICAL DETAILS OF THE EVOLUTIONARY OPTIMIZATIONS

The performance critical parts of the numerical framework (filling of the field-susceptibility matrices, numerical double-integration of the nanostructure volume Eq. (S.11)) are written in parallelized fortran using "openmp", all interfacing is written in python. The inversion problem is solved using the LU implementation in "scipy".

We use the open-source "paGMO" library, which provides a powerful toolbox for evolutionary optimization.[S5] In particular, we use the "pyGMO" python interface to paGMO and its implementation of the "jDe" differential evolution algorithm for single-objective problems.[S6] We use the "/rand/1/exp" parameter auto-adaptation scheme with otherwise default configuration. For the multi-objective example, we use the "moead" algorithm with "low discrepancy" weight generation and weighted objective decomposition.

## VII. ANALYSIS OF EVOLUTIONARY OPTIMIZATION CORRAL

In this section we discuss the gold-structure found by evolutionary optimization (EO). The goal was to obtain a maximum ratio of magnetic over electric decay rate enhancement. The generated corral-like structure is not of perfect symmetry, which we attribute to a not entirely finished convergence (see also main text). However, the principle idea, which the algorithm seems to "have in mind", is obvious: it consists of a thin outer circle and a broader inner one. The inner one might actually also be separated in two thin circles of different radius.

Hence, following this analysis of the geometry, we can divide the gold blocks in three circles: "Outer", "first inner" and "second inner". We categorized the blocks in these three groups (blue, green and orange colors in figure S.11), using their distance to the origin as selection criterion. To obtain the idealized version of the structure, we homogeneously redistribute the gold pillars in each group on perfect circles. As radius for each circle we use the average distance to the origin of all blocks in each of the three ensembles.

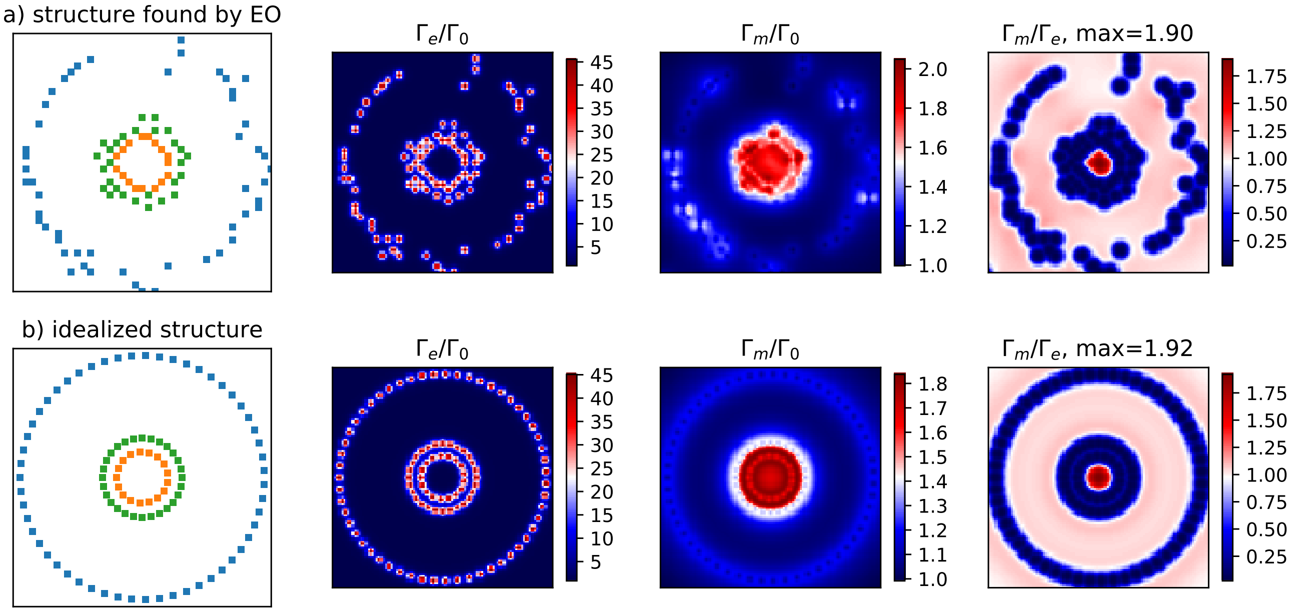


FIG. S.11. a) from left to right: Top view of structure as found by EO, electric dipole decay rate, magnetic dipole decay rate and the ratio $\Gamma_m/\Gamma_e$. b) same for an idealized version of the structure, consisting of three rings of equally spaced gold blocks. All plots show areas of $800 \times 800\,\mathrm{nm}^2$. Each scatter-point in the left plots correspond to a $20 \times 20 \times 60\,\mathrm{nm}$ gold pillar.

As can be seen in figure S.11, the results are qualitatively very similar (which is not really surprising). Yet, most importantly, the maximum of the ratio $\Gamma_m/\Gamma_e$ increases by only around 1 % if the residual disorder in the structure generated by evolutionary optimization is eliminated. We conclude that the optimization algorithm found a solution which is very close to ideal – despite the seemingly large amount of disorder.

## VIII. EVOLUTIONARY OPTIMIZATION – OPTIMIZE FOR DIAGONAL DIPOLE ORIENTATION

To demonstrate that the evolutionary optimization approach is not restricted to problems of high symmetry, we re-run the optimization of the main paper with a different dipole orientation. Instead of a dipole transition along $OZ$, we now search for a geometry that maximizes the ratio between magnetic and electric decay rate for an emitter oriented along the diagonal ($(x, y, z) = (1, 1, 1)$) with respect to the structure plane. The emitter is again placed at $(0, 0, 80)$ nm, hence 20 nm above the top surface of the planar nanostructure.

The optimum structure is shown in figure S.12a, its electric and magnetic decay rates as well as the ratio $\Gamma_m/\Gamma_e$ are shown in b)-d). Again, a structure with two functional components is found: An inner block of material, which enhances $\Gamma_m$ due to the dielectric contrast as well as an outer resonator, which further boosts the magnetic decay rate via its standing wave pattern (see Fig S.12e). Interestingly, the structure is not cylinder symmteric anymore, which is a result of the tilted radiation pattern of the diagonal dipole emitter. A rotation of the outer resonator by 90° (Fig S.12g) demonstrates, that in this case the enhancement of the magnetic decay rate is lower. Hence the magnetic versus electric decay enhancement for the specific dipole orientation is only optimal if the material is dispersed in an appropriate way around the quantum emitter. Figure S.12f) and h) show profiles across the center of the resonator, as indicated by dashed lines in e), respectively g).

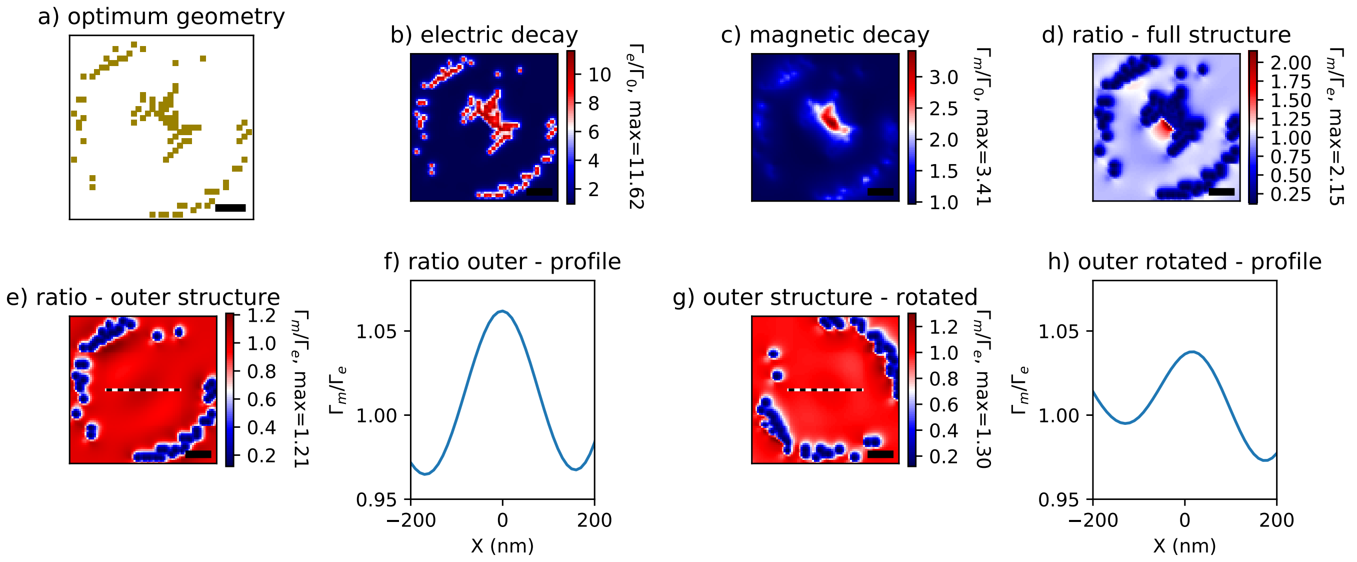


FIG. S.12. a-d): Top view of structure as found by EO, electric dipole decay rate, magnetic dipole decay rate and the ratio $\Gamma_m/\Gamma_e$. e-f) show the ratio of decay rates on the outer structure only. g-h) show $\Gamma_m/\Gamma_e$ for the outer structure (as in e), but rotated by 90° around the origin. f) and h) show profiles along the dashed lines in e), respectively g). All plots show areas of $800 \times 800\,\text{nm}^2$ with scale bars of 100 nm length. Each scatter-point in a) correspond to a $20 \times 20 \times 60$ nm gold pillar.

## IX. EVOLUTIONARY MULTI-OBJECTIVE OPTIMIZATION: OPTIMIZE AT TWO POSITIONS

To further demonstrate the versatility of the technique, we demonstrate here that also evolutionary multi-objective optimization (EMO) is possible with the formalism. For the demonstration we optimize the decay-rate ratio $\Gamma_m/\Gamma_e$ at two positions simultaneously, which we fix to $\mathbf{r}_1 = (-150, 0, 80)$ and $\mathbf{r}_2 = (+150, 0, 80)$ (in nm), for a dipole orientation along $Z$. The dipole emitters are hence positioned 20 nm above the structure. The latter is again composed of 100 gold pillars of $20 \times 20 \times 60\,\text{nm}^3$ each. We perform a Pareto multi-objective optimization. This means, using an evolutionary optimization algorithm we search all solutions which cannot be improved in one objective without worsening the other. From this finally obtained set of solutions (the "Pareto front"), we chose the candidate with most similar ratios at the both locations. Details on the employed multi-objective optimization scheme can be found in reference S7.

Figure S.13 shows the results of the optimization. The decay ratio $\Gamma_m/\Gamma_e$ of the full structure (Fig S.13c) is shown in figure S.13a). Like in the case of a single emitter, the structure is composed of small ring-formed structures around each optimization target location. They enhance the magnetic decay rate via their dielectric contrast. Furthermore, an outer oval resonator is formed, which additionally increases the magnetic decay rate at the two positions via its standing-wave pattern (see figure S.13b). Figure S.13d) shows the ratio of magnetic over electric decay rate along the dashed line indicated in b).

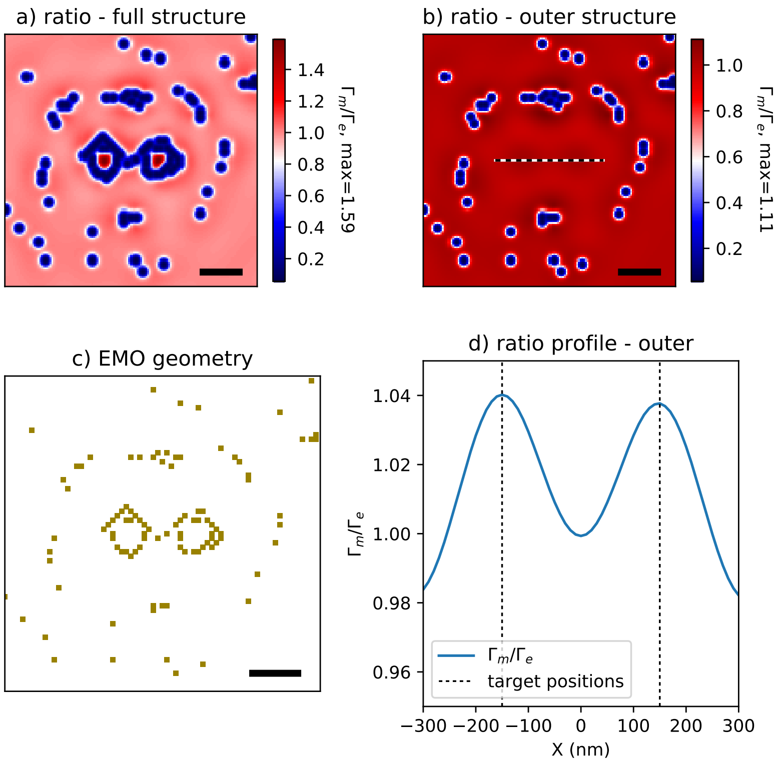


FIG. S.13. a) ratio $\Gamma_m/\Gamma_e$ for the full structure (which is shown in c). b) magnetic over electric decay rate ratio for the the outer resonator only. d) decay-rate ratio along the dashed line in b). The maps show areas of $1400 \times 1400\,\text{nm}^2$ with scale bars of 200 nm length. Each scatter-point in c) correspond to a $20 \times 20 \times 60$ nm gold pillar.

[S1] G. S. Agarwal, Physical Review A **11**, 230 (1975).
[S2] C. Girard, J.-C. Weeber, A. Dereux, O. J. F. Martin, and J.-P. Goudonnet, Physical Review B **55**, 16487 (1997).
[S3] O. J. F. Martin, C. Girard, and A. Dereux, Physical Review Letters **74**, 526 (1995).
[S4] C. Girard, T. David, C. Chicanne, A. Mary, G. C. des Francs, E. Bourillot, J.-C. Weeber, and A. Dereux, Europhysics Letters (EPL) **68**, 797 (2004).
[S5] F. Biscani, D. Izzo, and C. H. Yam, arXiv:1004.3824 [cs, math] (2010), arXiv:1004.3824 [cs, math].

[S6] S. M. Islam, S. Das, S. Ghosh, S. Roy, and P. N. Suganthan, IEEE Transactions on Systems, Man, and Cybernetics, Part B (Cybernetics) **42**, 482 (2012).

[S7] P. R. Wiecha, A. Arbouet, C. Girard, A. Lecestre, G. Larrieu, and V. Paillard, Nature Nanotechnology **12**, 163 (2017).
